# Supplementary material for: ARTiST: Automated Text Simplification for Task Guidance in Augmented Reality
Source: arXiv:2402.18797 source file (2024-02-29)
Supplement: Supplementary file 1 [file study.tex]

\section{Study Result}

\begin{figure}[h]
    \centering
    \includegraphics[width=0.5\linewidth]{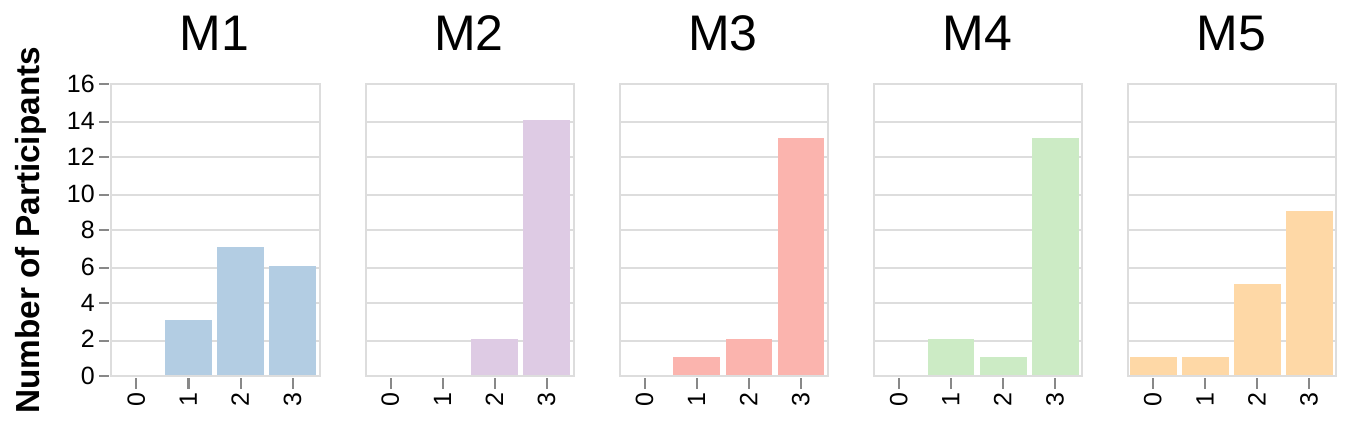}
    \caption{Study 2 result on the memory test.}
    \label{fig:study2-memory}
\end{figure}

\begin{figure}[t]
    \centering
    \includegraphics[width=0.5\linewidth]{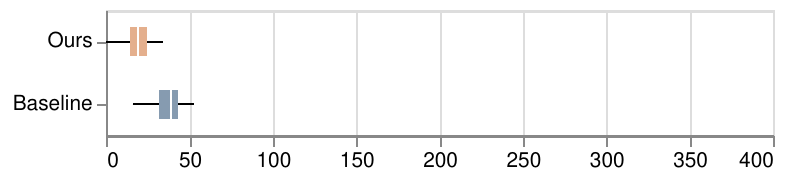}
    \caption{Task 1.1 NASA TLX overall task load.}
    \label{fig:study1.1-tlx-overall}
\end{figure}

\begin{figure}[t]
    \centering
    \includegraphics[width=0.5\linewidth]{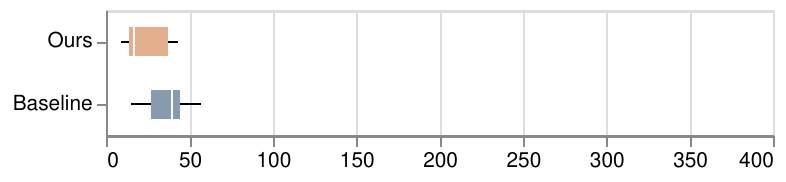}
    \caption{Task 1.2 NASA TLX overall task load}
    \label{fig:study1.2-tlx-overall}
\end{figure}

\begin{figure}[t]
    \centering
    \includegraphics[width=0.5\linewidth]{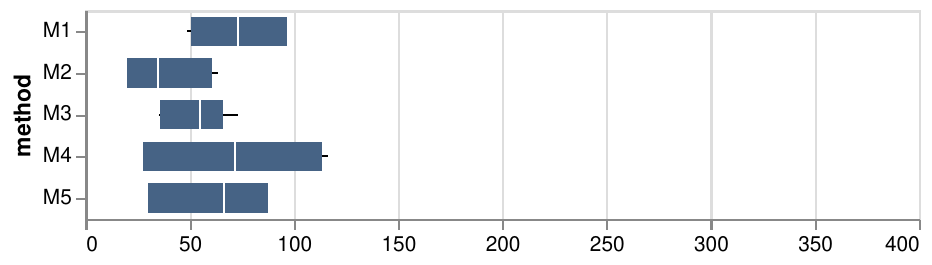}
    \caption{Study 2 NASA TLX task load}
    \label{fig:study2-tlx}
\end{figure}
